# Supplementary material for: ShARc: Shape and Appearance Recognition for Person Identification In-the-wild
Source: arXiv:2310.15946 source file (2023-10-24)
Supplement: Supplementary file 1 [file appendix.tex]

%\newpage

%\appendix

%\section{Appendix}\label{ablr}

%\subsection{Ablation Studies}
\appendix
\null
\begin{table*}
\vskip .375in
\begin{center}
  {\Large \bf \papertitle \\\textit{Supplementary Material} \par}
  % additional two empty lines at the end of the title
  \vspace*{24pt}
  {
  \large
  \lineskip .5em
  \begin{tabular}[t]{c}
     \vspace*{1pt}\\%This space will need to be here in the final copy, so don't squeeze it out for the review copy.
  \end{tabular}
  \par
  }
  % additional small space at the end of the author name
  \vskip .5em
  % additional empty line at the end of the title block
  \vspace*{12pt}
\end{center}
\end{table*}

\newpage

\input{tables/mevid_clothes}
Test
